# Supplementary material for: Structure of Core-Periphery Communities
Source: arXiv:2207.06964 source file (2022-07-14)
Supplement: Supplementary file 1 [file Appendixb0_influence_proof.tex]

\section{PROOF OF PROPOSITION \ref{prop:core_influence}}\label{proof:core_influence}

	Recall the definition of $S(y|\mu_c)$ given by	
	\begin{equation*}
	\begin{aligned}
	&S(y|\mu_c) = \sum_{z \in \Clw{y}} B(z|y) e^{ - \frac{\alpha}{\mu_c(z)} }.
	\end{aligned}
	\end{equation*}
	
	In addition, recall that objective function of the center agent is to maximize the total consumption utility of the community and the delay function is monotonic increasing with respect to rate allocation. By Proposition~\ref{prop:sufficient_budget}, we have all periphery agent connect to the core agent, and the core connect to all the periphery agents. Therefore,  increasing the budget from $M''_c$ to $M'_c$  would lead to that for all $y$ in the community,
	
	\begin{equation*}
		S(y|\mu'_c) > S(y|\mu''_c) 
	\end{equation*} 
	The increase in utility of content collected by the core agent won't effect the utility of other source. Therefore, we have that 
	\begin{equation*}
		U_{C,p}(\mu''_p(y)|\mu'_c,y) >  U_{C,p}(\mu''_p(y)|\mu''_c,y)
	\end{equation*} 
	
	Furthermore, since $S(y|\mu_c)$ increase for the periphery agent $y$, for the allocation of periphery agent to be optimal again, it has to satisfy Eq.~\eqref{eq:leaf_foc}. To satisfy Eq.~\eqref{eq:leaf_foc}, the periphery agent $y$ has to decrease the rate $\lambda(y)$ allocated for getting content outside the community. Therefore, we obtain that 
	 $$ \leafBudget - \lambda'(y)  >   \leafBudget - \lambda''(y).$$
	%Periphery agent behavior is defined by a utility-maximization problem.
        We then have that the  periphery agent $y$ will only do so if the utility increase by switching allocation. This implies that 
	 \begin{equation*}
	 	U_{C,p}(\mu'_p(y)|\mu'_c,y) >  U_{C,p}(\mu''_p(y)|\mu''_c,y). 
	 \end{equation*}
