# Supplementary material for: Structure of Core-Periphery Communities
Source: arXiv:2207.06964 source file (2022-07-14)
Supplement: Supplementary file 2 [file Appendixefficiency_proof.tex]

\section{PROOF OF PROPOSITION \ref{prop:social_welfare}}\label{proof:social_welfare}
In this appendix, we prove Proposition~\ref{prop:social_welfare}. The result of this proposition follow easily from Proposition~\ref{prop:stable_allocation}. To prove this result, we only need to show that the potential $G(\muc)$ captures the "social welfare" of all periphery agents, since we have shown in Proposition~\ref{prop:stable_allocation} that the unique Nash equilibrium is the global maxima for $G(\muc)$.

	Recall that the potential function $G(\muc)$ that characterize the interaction among agents is given as follow
	\begin{equation*}
	\begin{aligned}
	G(\muc) &=
	\sum_{y \in C_p} \sum_{z \in C_p \backslash\{y\}}  \delayCoreUtility{z}{y}\\
	&+ \sum_{y \in C_p} \delayUtility{z}{y}  + \sum_{y \in C_p}\alternative{\lambda(y)}.
	\end{aligned}
	\end{equation*}
	Using the definition for utility of periphery agents, we can rewrite the potential function $G(\muc)$ as follows,
	\begin{equation*}
	\begin{aligned}
	G(\muc) &= 
	\sum_{y \in C_p} \sum_{z \in C_p \backslash\{y\}}  \delayCoreUtility{z}{y}\\
	&+ \sum_{y \in C_p} \delayUtility{z}{y}  + \sum_{y \in C_p} \alternative{\lambda(y)} \\
		& = \sum_{y \in \leafSet}  \leafOptUtility{y}  \\
		& = \Phi(\muc)
	\end{aligned}
	\end{equation*}

        Recall the definition of the strategy space $\allstrategySpace$ of Appendix~\ref{proof:existence}, where we have shown that that there exists a unique Nash equilibrium $\mucs$ for the game of Section~\ref{sec:problem_formulation}, and we have that  $\mucs \in \allstrategySpace$. Furthermore, in Appendix~\ref{proof:existence} we have shown that
$$\mucs = \argmax_{\muc \in \possibleStrategy} G(\muc).$$
As we have obtained that $G(\muc) = \Phi(\muc)$, it follows that
$$\mucs = \argmax_{\muc \in \possibleStrategy} \Phi(\muc).$$
This completes the proof for Proposition~\ref{prop:social_welfare}.
