# Supplementary material for: Structure of Core-Periphery Communities
Source: arXiv:2207.06964 source file (2022-07-14)
Supplement: Supplementary file 3 [file Appendixfirst_order_condition.tex]

\section{FIRST ORDER CONDITION}\label{append:first_order_condition}
In this appendix, we will compute the first order optimal condition for periphery and core allocation problems. 

\subsection{First Order Condition}
In this section, we will compute the first order optimal condition for core and periphery allocation problems.

\subsubsection{First Order Condition for Core Agent Allocation}
Recall the core agent allocation problem 

\begin{equation*}
    \begin{split}
        &\max_{\mu(y_c)}\sum_{y \in \Com } \sum_{z \in \Cw{y}}  \\
        & \hspace{0.5in} \Bsbl B(z|y) e^{ - \alpha \left ( \frac{1}{\mu(z|y_c)} + \frac{1}{\mus(y_c|y)} \right)} -  c  \Bsbr I(\mu(z|y_c))I(\mus(y_c|y))
    \end{split}
\end{equation*}
subject to
$$ \sum_{y \in \Cwo} \mu(y|y_c) = b_0,$$
$$\mu(y|y_c) \geq 0.$$

Let $C(\mu(y_c))$ denote the objective function in the optimization problem above, the partial derivatives with respect to positive rate allocation are computed as follows
\begin{equation}
    \begin{split}
        \frac{dC(\mu(y_c))}{d\mu(y|y_c)}&=\frac{\alpha}{\mu^2(y|y_c)}e^{ - \frac{\alpha}{\mu(y|y_c)}}  \sum_{z \in \Cw{y} }  B(y|z) e^{  - \frac{\alpha}{\mu^*(y_c|z)} }
    \end{split}
\end{equation}

Note that by the formulation of indicator function. Any term with zero allocate rate would disappear in the objective function. By first order condition, we know that for an allocation to be optimal, the partial derivative with respect to the rate allocation of agents with positive positive value should converge to the same constant. In other word, by first order condition, we have for all agent $y \in \Com$ such that $\mu(y|y_c) > 0$, there exist some constant $f^{y_c}$
\begin{equation}
    \frac{dC(\mu(y_c))}{d\mu(y|y_c)} = f^{y_c}, \forall \mu(y|y_c)>0
\end{equation}

\subsubsection{First Order Condition for Periphery Agent Allocation}
Recall the periphery agent allocation problem 

\begin{equation*}
\begin{split}
    &\max_{\mu(y)} \Bsbl S(y_c|y)   e^{ - \frac{\alpha}{\mu(y_c|y)}}  - c(y_c) \Bsbr I(\mu(y_c|y))  \\
    &\hspace{0.5in} + \sum_{z \in \Cw{y}} \Bsbl B(z|y) e^{ - \frac{\alpha}{\mu(z|y)}} -   c\Bsbr I(\mu(z|y)) 
    + \beta \lambda(y)
\end{split}
\end{equation*}
subject to
$$ \sum_{z \in \Cw{y}} \mu(z|y)+ \mu(y_c|y) + \lambda(y) = B$$
$$\mu(z|y), \lambda(y), \mu(y_c|y) \geq 0.$$

Let $H(\mu(y))$ be the objective function in the optimization problem above, the partial derivatives with respect to positive rate allocation are computed as follows,
\begin{equation}
    \begin{split}
        \frac{dH(\mu(y))}{d\mu(y_c|y)}&=\frac{\alpha}{\mu^2(y_c|y)}e^{ - \frac{\alpha}{\mu(y_c|y)}}  \sum_{z \in \Cw{y}}  B(z|y) e^{  - \frac{\alpha}{\mu(z|y_c)} }\\
        \frac{dH(\mu(y))}{d\mu(z|y)}&=\frac{\alpha}{\mu^2(z|y)}e^{ - \frac{\alpha}{\mu(z|y)}}   B(z|y)\\
        \frac{dH(\mu(y)))}{d\lambda(y)}&=\beta
    \end{split}
\end{equation}

By first order condition, we have 
\begin{equation}
    \frac{dH_{y}(\mu(y))}{d\mu(y_c|y)} = \frac{dH_{y}(\mu(y))}{d\lambda(y)} = \frac{dH_{y}(\mu(y))}{d\mu(z|y)} = \beta, \forall \mu(y_c|y), \mu(z|y)> 0
\end{equation}
