# Supplementary material for: Structure of Core-Periphery Communities
Source: arXiv:2207.06964 source file (2022-07-14)
Supplement: Supplementary file 4 [file Appendixintermediate_result.tex]

\section{INTERMEDIATE RESULT}\label{Append:intermediate_result}
In this appendix, we will establish the intermediate results we use to prove our proposition.

\begin{lemma}\label{lemma:concavity}
    Under assumption \ref{concave_assumption}, the optimization problems that characterize core and periphery agent's allocation are concave.
\end{lemma}
\begin{proof}
Let's consider the delay factor $e^{-\frac{\alpha}{\mu}}$ and denote it as $D(\mu)$. To show this lemma, it is enough to show $D(\mu)$ is concave, since the objectives function of core and periphery agents are sum of delay factor up to difference of a constant factor and the sum of concave function is again concave.

The first and second derivative of the delay factor are computed as follow:
\begin{equation}
    \begin{split}
        \frac{dD(\mu)}{d\mu} &= \frac{\alpha}{\mu^2}e^{-\frac{\alpha}{\mu}}\\
        \frac{d^2D(\mu)}{d^2\mu} &= \frac{\alpha}{\mu^3}e^{-\frac{\alpha}{\mu}}(\frac{\alpha}{\mu}-2)
    \end{split}
\end{equation}
By assumption \ref{concave_assumption}, we have $\mu > \frac{\alpha}{2}$, which leads to $\frac{d^2D(\mu)}{d^2\mu} < 0$. Therefore, the delay factor is concave in the region we are considering the interaction.
\end{proof}
\begin{lemma}\label{lemma:bmin1}
There exist a finite positive $b^1$ such that if the budget of core agent $b_0 > b^1$, then agent, closer to the center of community, would benefit more from the content of core agent. In other word, given two leaf agents $y_i, y_j$
$$\|y_i - y_0\|<\|y_j - y_0\|$$
we have 
$$S(y_0|y_i) > S(y_0|y_j)$$
\end{lemma}

\begin{proof}
By assumption \ref{assump:benefit_rank}, we have that in the case without delay, agent closer to the center of community would benefit more from the content of the community. More precisely, for agents $y_i,y_j$, if 
$$\|y_i - \Icen \|<\|y_j - \Icen \|$$
then
$$\sum_{z \in \Com \backslash \{y_i\}} B(z|y_i)> \sum_{z \in \Com \backslash \{y_j\}}B(z|y_j)$$
Let
\begin{equation}\label{eq:delta}
    \begin{split}
        &\Delta = \min_{\cb{y_i,y_j| \|y_i - \Icen \| \neq \|y_j - \Icen \|}}\\
        &\hspace{0.5in}  \|\sum_{z \in \Com \backslash \{y_i\}} B(z|y_i) - \sum_{z \in \Com \backslash \{ y_j\}}B(z|y_j)\|
    \end{split}
\end{equation}
In other word, $\Delta$ is the minimum difference of consumption utility of any two agents in the community in the case without delay.

Since the delay factor of core agent getting content from periphery agent $y$ is a monotonic increasing function with respect to the allocation rate $\mu(y|y_0)$, we have $e^{\frac{-\alpha}{\mu(y|y_0)}} \xrightarrow{} 1, \text{ as } \mu(y|y_0) \xrightarrow{} \infty$. This means as the rate allocation increase, we can find a upper bound between the difference of the case with delay and the case without delay for each agent. Let $\epsilon_{y}$ be the upper bound of the difference between the case with delay and the case without delay for agent $y$. In other word, let

\begin{equation}
    \epsilon_{y} \geq 1 -  e^{\frac{-\alpha}{\mu(y|y_0)}}
\end{equation}

Then, we can find the maximum difference among all agent. In other word, find the agent that is effected by the delay the most and denote the its delay effect as $\epsilon^*$.

\begin{equation}\label{eq:epsilon}
    \epsilon^* = \max_{y \in \Com}\epsilon_{y}
\end{equation}

As $b_0 \xrightarrow{} \infty$,  $\epsilon^* \xrightarrow{} 0$.

Let's denote the number of periphery agent in the community as N. We can find a finite $b^1$ large enough such that $\Delta > N\epsilon^*$. Then, for all periphery agent $y_i,y_j$ in the community, we have 
\begin{equation}
    \begin{split}
        \sum_{z \in \Com \backslash \{y_i\}} B(z|y_i)e^{\frac{-\alpha}{\mu(z|y_0)}} - \sum_{z \in \Com \backslash \{y_j\}}B(z|y_j)e^{\frac{-\alpha}{\mu(z|y_0)}} &> \Delta \\
        & > N\epsilon^*
    \end{split}
\end{equation}
By equation\ref{eq:delta} and equation \ref{eq:epsilon}, we have 
\begin{equation}
    \begin{split}
        S(y_0|y_i) &> \sum_{z \in \Com \backslash \{y_i\}} B(z|y_i)e^{\frac{-\alpha}{\mu(z|y_0)}} - N\epsilon^* \\
        &> \sum_{z \in \Com \backslash \{y_j\}}B(z|y_j)e^{\frac{-\alpha}{\mu(z|y_0)}}\\
        &>S(y_0|y_j)
    \end{split}
\end{equation}

Therefore, we have 
$$S(y_0|y_i) > S(y_0|y_j)$$

\end{proof}

\begin{lemma}\label{lemma:bmin2}
For all agent y in the community, let $z^*_y = \max_z B(z|y)$. In other word, $z^*_y$ is the agent that produce content is of most beneficial to agent y.

There exist a finite positive $b^2$ such that if the budget of core agent $b_0 > b^2$, we have
$$S(y_0|y) > B(z^*_y|y)$$
This means that the core agent possess content is of the highest value to agent y.
\end{lemma}

\begin{proof}
In the case without delay, for all agent y in the community we have that 
$$\sum_{z \in \Com \backslash \cb{y}} B(z|y)> B(z^*_y|y) $$
Let $\Delta = \min_{y \in \Com} \sum_{z \in C \backslash \{y\}} B(z|y) - B(z^*|y)$. In other word, $\Delta$ is the minimum difference between the total utility of whole community content and utility of the highest valuable content for any agent in the community. 

As we establish in the proof of lemma \ref{lemma:bmin1}, for all positive $\epsilon$, we can find a positive finite $b^2$ large enough such that 
$$\sum_{z \in \Com \backslash \cb{y}} B(z|y) - S(y_0|y) < \epsilon$$
Therefore, we can make $b^2$ large enough such that we have $\epsilon < \Delta$. This leads to that for all agent y we have,
\begin{equation*}
    \begin{split}
        \sum_{z \in \Com \backslash \cb{y}} B(z|y) - S(y_0|y) &< \epsilon \\
        &<\Delta\\
        &\leq \sum_{z \in \Com \backslash \cb{y}} B(z|y) - B(z^*_y|y)
    \end{split}
\end{equation*}
Therefore, if $b_0 > b^2$, then we have for any agent y, 
$$S(y_0|y) > B(z^*_y|y)$$

\end{proof}
\begin{lemma}\label{lemma:periphery_agent_allocation}
Let $b_{min} = \max \{ b^1, b^2\}$
If 
$$b_0 > b_{min}$$
then for all agents $y_i, y_j$ in the community, if 
$$\|y_i - \Icen \| < \|y_j - \Icen \|$$
then we have 
$$\mu(y_0|y_i) > \mu(y_0|y_j)$$
\end{lemma}

\begin{proof}
Let $y_i, y_j$ be any two agents in the community. Without loss of generality, we assume that
$$\|y_i - y_0\|<\|y_j - y_0\|$$
Since $b_0 > b^1$, by Lemma \ref{lemma:bmin1}, we have that $S(y_0|y_i) > S(y_0|y_j)$. Or equivalently,
$$\sum_{z \in \Com \backslash\{y\}}  B(z|y_i) e^{  - \frac{\alpha}{\mu(z|y_0)} } > \sum_{z \in \Com \backslash\{y\}}  B(z|y_j) e^{  - \frac{\alpha}{\mu(z|y_0)} }$$

Recall the partial derivative with respect to $\mu(y_0|y)$ in the optimization is 
$$ \frac{dH(\mu(y))}{d\mu(y_0|y)}=\frac{\alpha}{\mu^2(y_0|y)}e^{ - \frac{\alpha}{\mu(y_0|y)}} S(y_0|y)$$
For the allocation to be optimal, the allocation need to satisfy the first order condition. By lemma \ref{lemma:bmin2}, we have that for all agent periphery agents $y$, $\mu(y_0|y) > 0$. This means that the first order condition with respect to $\mu(y_0|y)$ is $\frac{dH(\mu(y))}{d\mu(y_0|y)} = \beta$. Because $\beta$ is same for all agents, we have 

\begin{equation}
    \begin{split}
         \frac{\alpha}{\mu^2(y_0|y_i)}e^{ - \frac{\alpha}{\mu(y_0|y_i)}}  S(y_0|y_i)
        = 
         \frac{\alpha}{\mu^2(y_0|y_j)}e^{ - \frac{\alpha}{\mu(y_0|y_j)}}  S(y_0|y_j)
    \end{split}
\end{equation}

Since $\|y_i - \Icen \| < \|y_j - \Icen \|$ by assumption, by lemma \ref{lemma:bmin1}, we have
\begin{equation}
    S(y_0|y_i) > S(y_0|y_j)
\end{equation}
This leads to
$$\mu(y_0|y_i) > \mu(y_0|y_j)$$
\end{proof}
\begin{lemma}\label{lemma:core_allocation}
If $b_c$ satisfy the condition in lemma \ref{lemma:periphery_agent_allocation},
then for arbitrary agents $y_i, y_j$ in the community such that
$$\|y_i - \Icen \| < \|y_j - \Icen \|$$
we have 
$$\mu(y_i|y_0) > \mu(y_j|y_0)$$
\end{lemma}

\begin{proof}
Let $y_i$, $y_j$ be two arbitrary agents such that 
$$\|y_i-y_0\| < \|y_j-y_0\|$$
To show the result of this lemma, it is enough to show the following
\begin{equation}\label{eq:lemma4_sufficient_condition}
    \sum_{z \in \Com \backslash \{y_i\}} B(y_i|z)e^{\frac{-\alpha}{\mu(y_0|z)}}> \sum_{z \in \Com \backslash \{y_j\}} B(y_j|z)e^{\frac{-\alpha}{\mu(y_0|z)}}
\end{equation}
then, first order condition condition would imply the optimal allocation has 
$$\mu(y_i|y_0) > \mu(y_j|y_0)$$

Recall $\delta$ is the distance of any consecutive agents in the content space of the community and it determine the community density. As $\delta$ decrease, the community density increase.
In addition, under the case without delay, by assumption \ref{assump:production_strategy}, we have that 
$ \sum_{z \in \Com \backslash \{y_i\}} B(y_i|z)> \sum_{z \in \Com \backslash \{y_j\}} B(y_j|z)$. Therefore, this lemma aim to establish that under the condition described, this relation is also true for the case with delay. To show this, we will use the result established in lemma \ref{lemma:periphery_agent_allocation},i.e. $\mu(y_0|y_i) > \mu(y_0|y_j)$. Using these results, we partition the community content interval and compare the utility of agents in each section. We will see that so long as the community is dense enough ($\delta$ small enough), then we obtain the relation in equation \ref{eq:lemma4_sufficient_condition}.

Let $\muc^*$ be the rate allocation vector of agents defined earlier. Without loss of generality, let's assume that content interval of the community is given by the following
$$I_C = (-L_C, L_C) \mbox{ and } mid(I_C) = 0$$
Then$\|y_i-\Icen \| < \|y_j-\Icen \|$ leads to three possible cases:\\
case 1: $y_i$ and $y_j$ are in the same side of the community, (0,$L_C$)\\
case 2: $y_i$ and $y_j$ are in the same side of the community, ($-L_C$,0)\\
case 3: $y_i$ and $y_j$ are on different side of the community

The proof for these three cases are similar. Therefore, we will only construct proof for one of the case above. Let's consider the case $y_i$, and $y_j$ are on the same half interval, (0,$L_C$). We can partition the community interval into the following sections:\\
\begin{equation*}
    \begin{split}
        S_1 &= (x^*(y_j),L_C)\\
        S_2 &= (\frac{x^*(y_j)-x^*(y_i)}{2},x^*(y_j))\\
        S_3 &= (x^*(y_i),\frac{x^*(y_j)-x^*(y_i)}{2})\\
        S_4 &= (x^*(y_i)+x^*(y_j)-L_C,x^*(y_i))\\
        S_5 &= (-L_C,x^*(y_i)+x^*(y_j)-L_C)
    \end{split}
\end{equation*}
Then, let's consider the difference of utility in each sections above.\\
Let $N(S_i)$ denote the set of leaf agents in the interval $S_i$, $\|N(S_i)\|$ is the number of leaf agents in $S_i$, and let $\Delta_{S_i}$ denote the difference of utility between $y_i$ and $y_j$ in interval $S_i$. Further, the $\Delta_{S_i}$ is given by 
\begin{equation*}
    \begin{split}
        \Delta_{S_i} &=\sum_{z \in N(S_i)} [B(y_i|z)-B(y_j|z)|z)] e^{-\frac{\alpha}{\mu(y_0|z)}} \\
        &= \sum_{z \in N(S_i)} [g(x^*(y_i)|y_i)f(x^*(y_i)|z)-\\
        &\hspace{0.5inch} g(x^*(y_j)|y_i)f(x^*(y_j)|z)] e^{-\frac{\alpha}{\mu(y_0|z)}} 
    \end{split}
\end{equation*}

We will show that the overall difference of $\Delta_{S_4}$ and $\Delta_{S_1}$ is positive,i.e,
$$\Delta_{S_4} + \Delta_{S_1} > 0$$

We know that the distance between consecutive agent is the same on the interval, and by construction, we have
$$\|S_1\| = \|S_4\|$$
which implies 
$$\|N(S_1)\| = \|N(S_4)\|$$
Let $J = \|N(S_1)\| = \|N(S_4)\|$. By construction of the information community in section \ref{sec:background} and the production strategy of agent \ref{assump:production_strategy}, we know that the distance between $x^*(y_j)$ to agents in $S_1$ are multiple of $\delta$ in addition to some distance $\epsilon_{s_1}$ to the first agent, where $\epsilon_{s_1} < \delta$.
Similarly for $S_4$. We can rewrite $\Delta_{S_1}$ and $\Delta_{S_4}$ as 
\begin{equation*}
    \begin{split}
        \Delta_{S_1} &= - \sum_{k=0}^J [g(x^*(y_j)|y_j)f(k\delta + \epsilon_{s_1} )\\
        &-g(x^*(y_i)|y_i)f(x^*(y_j)-x^*(y_i)+k\delta + \epsilon_{s_1}) ]e^{-\frac{\alpha}{\mu(y_0|x^*(y_j)+k\delta + \epsilon_{s_1})}}
    \end{split}
\end{equation*}
\begin{equation*}
    \begin{split}
        \Delta_{S_4} &= \sum_{k=0}^J [g(x^*(y_i)|y_i)f(k\delta + \epsilon_{s_4})\\
        &-g(x^*(y_j)|y_j)f(x^*(y_j)-x^*(y_i)+k\delta + \epsilon_{s_4})] e^{-\frac{\alpha}{\mu(y_0|x^*(y_i)-k\delta + \epsilon_{s_4})}}
    \end{split}
\end{equation*}

Then, with the result from assumption \ref{assump:production_strategy}, we have 
$$g(x^*(y_i)|y_i) > g(x^*(y_j)|y_j)$$
and by lemma \ref{lemma:periphery_agent_allocation}, we have that
$$e^{-\frac{\alpha}{\mu(y_0|x^*(y_j)+k\delta \pm \epsilon_{s_1})}}<e^{-\frac{\alpha}{\mu(y_0|x^*(y_i)-k\delta\pm \epsilon_{s_4})}}$$

Since $\epsilon_{s_1}, \epsilon_{s_4} < \delta$, we can make $\delta$ small enough such that the small misalignment $\epsilon_{s_1}, \epsilon_{s_4}$ does not effect the comparison of each term in the sum. Let $\delta_0$ be be the term that satisfy this condition. In other word, if $\delta < \delta_0$, then we have the following for each term of the two sum
\begin{equation*}
    \begin{split}
        &[g(x^*(y_i)|y_i)f(k\delta \pm \epsilon_{s_4})\\
        &-g(x^*(y_j)|y_j)f(x^*(y_j)-x^*(y_i)+k\delta + \epsilon_{s_4})] e^{-\frac{\alpha}{\mu(y_0|x^*(y_i)-k\delta + \epsilon_{s_4})}} \\
        &>\\
        &[g(x^*(y_j)|y_j)f(k\delta + \epsilon_{s_1} )\\
        &-g(x^*(y_i)|y_i)f(x^*(y_j)-x^*(y_i)+k\delta + \epsilon_{s_1}) ]e^{-\frac{\alpha}{\mu(y_0|x^*(y_j)+k\delta + \epsilon_{s_1})}}
    \end{split}
\end{equation*}

This means that each term in $\Delta_{S_4}$ is strictly larger than its corresponding term in $\Delta_{S_1}$. Therefore, we have
\begin{equation}\label{s14}
    \Delta_{S_1} + \Delta_{S_4} > 0    
\end{equation}

By similar argument, we can get
\begin{equation}\label{s23}
    \Delta_{S_2} + \Delta_{S_3} > 0    
\end{equation}

Now, let's consider the last interval $S_5$
\begin{equation*}
    \begin{split}
        \Delta_{S_5} &= \sum_{z \in N(S_5)} [B(y_i|z)-B(y_j|z)]e^{-\frac{\alpha}{\mu(y_0|z)}} 
    \end{split}
\end{equation*}
Since $y_i$ is closer to agents in $N(S_5)$ than $y_j$ by construction, we have 
$$B(y_i|z) > B(y_j|z) \text{  ,   } \forall z \in N(S_5)$$
This immediately leas to, 
\begin{equation}\label{s5}
    \Delta_{S_5} > 0
\end{equation}

Combining the results \ref{s14}, \ref{s23}, \ref{s5} above, we get
$$\Delta_{S_1}+\Delta_{S_2}+\Delta_{S_3}+\Delta_{S_4}+\Delta_{S_5}>0$$
Therefore, we obtain 
\begin{equation*}
    \sum_{z \in \Com \backslash \{y_i\}} B(y_i|z)e^{\frac{-\alpha}{\mu(y_0|z)}}> \sum_{z \in \Com \backslash \{y_j\}} B(y_j|z)e^{\frac{-\alpha}{\mu(y_0|z)}}
\end{equation*}
And the result of the lemma is immediately followed from first order condition.

\end{proof}
