# Supplementary material for: Structure of Core-Periphery Communities
Source: arXiv:2207.06964 source file (2022-07-14)
Supplement: Supplementary file 5 [file Appendixleaf_consumption_proof.tex]

\section{PROOF OF PROPOSITION \ref{prop:periphery_consumption}}\label{proof:periphery_consumption}
In this appendix, we will give a proof to Proposition \ref{prop:periphery_consumption}. To show this proposition, we will first show that the closer an periphery agent to the center of community, the more rate the agent allocates to participating the community.

\begin{lemma}\label{lemma:leaf_budget_dist}
	Let  $\muc^* = (\mu_c^*,\muc^*_p)$ be a stable allocation as given in Proposition~\ref{prop:sufficient_budget}.
	If for two periphery agents $y,y' \in \leafSet$ we have
	$||y - \Cc || < ||y' - \Cc ||$,
	then we have that  
	$$ \leafBudget - \lambda^*(y)  >   \leafBudget - \lambda^*(y').$$
\end{lemma}

\begin{proof}
    Let's start with two periphery agents $y$ and $y'$ such that 
	$$\|y - \Icen\| = \| y' - \Icen \|$$
	In this case, we have that 
	$$\leafAllocation{y} = \leafAllocation{y'},$$
	and 
	$$\lambda(y) = \lambda(y'),$$
	and
	$$\mu(y_c|y) = \mu(y_c|y').$$
	Furthermore, by first order condition as given in Eq.~\eqref{eq:leaf_foc}, we have that 
	\begin{equation*}
	S(y|y_c)e^{\frac{-\alpha}{\mu(y_c|y)}}\frac{\alpha}{\mu^2(y_c|y)} = r_0B_0e^{\frac{-\alpha}{\lambda(y)}} \frac{\alpha}{\lambda^2(y)}
	\end{equation*}
	As we move agent $y$ toward the center of community, by Proposition~\ref{lemma:core_respond}, we have that the utility of content collected by the core agent $y_c$, $S(y_c|y)$, would increase. Let's denote the increased utility agent $y$ get from the core as $S'(y_c|y)$, then we have the following.
	\begin{equation*}
	S'(y|y_c)e^{\frac{-\alpha}{\mu(y_c|y)}}\frac{\alpha}{\mu^2(y_c|y)} > r_0B_0e^{\frac{-\alpha}{\lambda(y)}} \frac{\alpha}{\lambda^2(y)}
	\end{equation*}
	For the allocation of periphery agent $y$ to be optimal, it has to satisfy the first order condition and thus, would switch to an new allocations $\mu'_p(y)$ such that  
	$$\mu'(y_c|y) > \mu(y_c|y),$$
	and
	$$\lambda'(y) < \lambda(y)$$
	Therefore, we have that 
	$$\lambda'(y) < \lambda(y) = \lambda(y')$$
	Therefore, as $y$ closer to the center of community, i.e,
	$$\|y - \Icen\| < \| y' - \Icen \|$$
	then, we have 
	$$\lambda(y) < \lambda(y').$$
	Since all periphery agents have the same budget, this leads to the result of the proposition
	$$M_p - \lambda(y) > M_p -\lambda(y').$$
\end{proof}

%\section{Proof of Proposition \ref{prop:structure}}
%Here, we show that an iterative update process, that converge to the unique stable allocation, has the structural properties given in the proposition would preserve in each iteration. Therefore, the stable allocation in the end has the same structural property. 
%\input{content/appendix/centralized_proof3.tex}

Now that we have established the Lemma~\ref{lemma:leaf_budget_dist}, we shall prove Proposition~\ref{prop:periphery_consumption}.

\begin{proof}
	Recall that the utility that agent $y$ get from the community is given as follows.
	\begin{equation*}
	\begin{split}
	& \leafCommUtility{y} \\
	= &  \sum_{z \in \Clw{y}} \delayCoreUtility{z}{y}  \\
	& + \sum_{z \in \Clw{y}} \delayUtility{z}{y}.
	\end{split}
	\end{equation*}
	Furthermore,  recall that the complete utility function of the periphery agent is given as follows.
	\begin{equation*}
	\begin{split}
	&U(y|\coreRateVec,\leafRateVec{y}) = \\
	& \sum_{z \in \Cw{y}} \delayCoreUtility{z}{y}  \\
	&\hspace{0.3in} + \delayUtility{z}{y}
	+ \alternative{\lambda(y)}.
	\end{split}
	\end{equation*}
	Let $y$ and $y'$ be two periphery agents as given in this proposition. We have 
	$$\|y-\Cc\| < \|y' - \Cc\|$$
	From Lemma~\ref{lemma:leaf_budget_dist}, we have that 
	$$\lambda(y) < \lambda(y')$$
	Suppose $y = y'$. In other word, let's suppose y and y' have the same center of interest. Then we have the following
	$$U(y|\coreRateVec,\leafRateVec{y}) = U(y'|\coreRateVec,\leafRateVec{y'})$$
	$$\leafCommUtility{y} = \leafCommUtility{y'}$$
	and
	$$\lambda(y) = \lambda(y')$$
	As we move agent $y$ toward the center of community, the rate allocation of $y$ for getting content from outside the community decrease. However, by formulation of the problem, the behavior of agent $y$ is defined by maximizing its own utility. Therefore, $y$ would decrease its rate allocation for the content source outside the community only if $y$ can obtain a larger utility. Therefore, we have that if $$\|y-\Cc\| < \|y' - \Cc\|,$$
	then
	$$\leafCommUtility{y} >\leafCommUtility{y'}$$
\end{proof}
