# Supplementary material for: Structure of Core-Periphery Communities
Source: arXiv:2207.06964 source file (2022-07-14)
Supplement: Supplementary file 6 [file Appendixlower_bound_participation.tex]

\section{PROOF OF PROPOSITION \ref{prop:participate_condition}}\label{proof:participate_condition}

We prove Proposition \ref{prop:participate_condition} by contradiction.
	Suppose that Proposition \ref{prop:participate_condition} is not true, then there exists an agent $y$ such that no matter how large the rate budget $\leafBudget$ is, we have that for the optimal allocation $\optLeafAllocation{y}$ of agent $y$ that
	$$\sum_{z \in C} \mu^*(z|y) = 0.$$
	In other words, the best strategy for agent $y$ is to not participate in the community. There are two possible reasons for this: Case 1) agent $y$ does not not get any content and we have that $\lambda(y) = 0$, and Case 2) agent $y$x gets only content from content platforms outside the community and $\lambda(y) = \leafBudget$. We analyze these two cases below. 
	
We first consider the case where $\lambda(y) = 0$. 
	By Assumption~\ref{ass:positive_utility}, there exists at least one agent $z$ such that 
	$$B(z|y) - c >0.$$
	This implies that there exist a finite $M$ such that 
	$$B(z|y)e^{-\frac{\alpha}{M}} - c \geq  0.$$

	Let $M^*$ be the smallest $M$ that achieve this property, i.e,
	$$M^* = \min\{M > 0 |B(z|y)^{-\frac{\alpha}{M}} - c \geq  0\}.$$
	
	It the follows that if $M_p > M^*$, then agent $y$ gets a  positive utility from following agent $z$ and the $\optLeafAllocation{y}$ such that
        $$\sum_{z \in C} \mu^*(z|y) = 0$$
        is not optimal. This leads to a contraction to the assumption that the allocation  $\optLeafAllocation{y}$ is optimal. 
	
        Next we consider the case where $\lambda(y) = \leafBudget$. 
        By Assumption~\ref{ass:positive_utility}, there exists at least one agent $z$ such that 
	$$B(z|y) - c >0.$$
        It then follows that there exists an agent $z$ and $M > 0$ such that 
	$$B(z|y)e^{-\frac{\alpha}{M}} - c = u > 0.$$
        Without loss of generality, assume that $\leafBudget > M$, and 
	consider decreasing the rate $\lambda(y)$  by $M$.
	The difference in the utility obtained by agent $y$ is then given by
	\begin{equation*}
		r_0 B_0 e^{-\frac{\alpha}{M_p}} - r_0 B_0 e^{-\frac{\alpha}{M_p-M}}
	\end{equation*}
	
	By Lemma~\ref{lemma:potential_game_convexity}, the function $e^{-\frac{\alpha}{x}}$ is strictly concave for $ x \in \strategySpace_p$, and we have that 
	\begin{equation*}
	\begin{aligned}
			B_0 e^{-\frac{\alpha}{M_p}} - B_0 e^{-\frac{\alpha}{M_p-M}}
	\leq M \frac{\alpha}{(M_p)^2}B_0 e^{-\frac{\alpha}{M_p}}.
	\end{aligned}
	\end{equation*}
        As we have that
	
	$$\lim_{M_p \to \infty} \frac{\alpha}{M_p^2}B_0 e^{-\frac{\alpha}{M_p}}  = 0,$$
	it follows that there exists a finite $M_p^*$ such that 
	\begin{equation*}
		\begin{aligned}
		&B_0 e^{-\frac{\alpha}{M_p^*}} - B_0 e^{-\frac{\alpha}{M_p^*-M}}
		< M \frac{\alpha}{(M_p^*)^2}B_0 e^{-\frac{\alpha}{M_p^*}} 
		< u.
		\end{aligned}
	\end{equation*}
	This implies that for  $M_p > M_p^*$, then $y$ can increase its  utility by setting $\mu(z|y) = M$ and $\lambda(y) =  M_p^* - M$.
This leads to a contraction to the assumption that the allocation  $\optLeafAllocation{y}$ is optimal. 

This completes the proof of the proposition.
