# Supplementary material for: Structure of Core-Periphery Communities
Source: arXiv:2207.06964 source file (2022-07-14)
Supplement: Supplementary file 7 [file centralized_proof.tex]

%Let $G(\muc)$ be the objective function in the optimization problem above, we compute the partial derivative with respect to each rate 
%\begin{equation}
%    \begin{split}
%        \frac{dG(\muc)}{d\mu(y|y_c)}&=\frac{\alpha}{\mu^2(y|y_c)}e^{ - \frac{\alpha}{\mu(y|y_c)}}  \sum_{z \in \Com \backslash\{y\}}  B(y|z) e^{  - \frac{\alpha}{\mu(y_c|z)} }\\
%        \frac{dG(\muc)}{d\mu(y_c|y)}&=\frac{\alpha}{\mu^2(y_c|y)}e^{ - \frac{\alpha}{\mu(y_c|y)}}  \sum_{z \in \Com \backslash\{y\}}  B(z|y) e^{  - \frac{\alpha}{\mu(z|y_c)} }\\
%        \frac{dG(\muc))}{d\lambda(y)}&=\beta
%    \end{split}
%\end{equation}
%
%
%\subsection{First Order condition}
%By First Order condition, we know that partial derivative of all the terms(with positive allocation) should converge to the same constant for each agent. In other word, we have for $\forall y \in C$
%$$\frac{dG(\muc)}{d\mu(y|y_c)} =\frac{dG(\muc)}{d\mu(y_c|y)} = \frac{dG(\muc)}{d\lambda(y)} = \beta, \mu(y_c|y), \lambda(y) > 0$$

\newpage 

\section{Global Optimization Characterize the Global Allocation}
Let $\muc$ denote the allocation of all agents in the community

\begin{equation}
    \begin{split}
          \max_{\muc}  \sum_{y \in \Com} \sum_{z \in \Com \backslash\{y\}}  [  B(z|y) e^{ - \frac{\alpha}{\mu(z|y_c)} - \frac{\alpha}{\mu(y_c|z)} }  -  c ] I(\mu(z|y_c)) + \beta \lambda(y),
    \end{split}
\end{equation}
such that
$$ \sum_{y \in \Com} \mu(y|y_c) = b_c,$$
$$ \mu(y_c|y) + \lambda(y) = B, \forall y \in \Com$$
and
$$\mu(y|y_c), \mu(z|y), \lambda(y) \geq 0.$$

\subsection{Stable Allocation}
Let $\muc^*$ be a set of allocation for all periphery agents and core agents with the following properties:

\begin{enumerate}
	\item the allocation is symmetric between core and periphery,i.e, $\mu(y_c|y) = \mu(y|y_c)$
	\item the allocation is symmetric around core of community,i.e, if $\|y-\Icen\| =\|y' - \Icen \|$, then $\mu(y_c|y') = \mu(y_c|y)$
	\item the closer an periphery agent is to the core of community, the more rate he would allocate to the core. In other word, $\|y-\Icen\| <\|y' - \Icen \|$, then $\mu(y_c|y') > \mu(y_c|y)$
\end{enumerate}

\begin{prop}
	Property (3) is necessary condition for allocation $\muc^*$ to be stable
\end{prop}

To simplify the notation, we can write 
\begin{equation}
	\mu(y|y_c) = \mu(y_c|y) = \mu_y
\end{equation}

This is true because of property (1)

\begin{proof}
	Let $\muc’$ be an optimal allocation with a pair of  agent $y_1,y_2$ such that
	$$\|y_1 - \Icen\|<\|y_2 - \Icen \|$$
	and
	$$\mu_{y_1}<\mu_{y_2}$$
	
	We want to show that by swapping the rate of $y_1 \& y_2$, we can get a bigger utility.

	Let's compute the utility associate with $y_1, and y_2$. Because the term associate with alternative is identical for all  agents, swapping the allocation does not effect the total sum. Therefore, we will drop the alternative in the analysis later for simplicity.
	
	\begin{equation}\label{uy1}
	\begin{split}
	\sum_{z \in  \Com \backslash \{y_1,y_2\}}B(z|y_1) e^{-\frac{\alpha}{\mu_z} -\frac{\alpha}{\mu_{y_1}}} + B(y_2|y_1)e^{-\frac{\alpha}{\mu_{y_2}} -\frac{\alpha}{\mu_{y_1}}} \\
	+ \sum_{z \in  \Com \backslash \{y_1,y_2\}}B(y_1|z) e^{-\frac{\alpha}{\mu_z} -\frac{\alpha}{\mu_{y_1}}} + B(y_1|y_2)e^{-\frac{\alpha}{\mu_{y_2}} -\frac{\alpha}{\mu_{y_1}}} \\
	\end{split}
	\end{equation}
	
	\begin{equation}\label{uy2}
	\begin{split}
	\sum_{z \in  \Com \backslash \{y_1,y_2\}}B(z|y_2) e^{-\frac{\alpha}{\mu_z} -\frac{\alpha}{\mu_{y_2}}} + B(y_1|y_2)e^{-\frac{\alpha}{\mu_{y_2}} -\frac{\alpha}{\mu_{y_1}}} \\
	+ \sum_{z \in  \Com \backslash \{y_1,y_2\}}B(y_2|z) e^{-\frac{\alpha}{\mu_z} -\frac{\alpha}{\mu_{y_2}}} + B(y_2|y_1)e^{-\frac{\alpha}{\mu_{y_2}} -\frac{\alpha}{\mu_{y_1}}} \\
	\end{split}
	\end{equation}
	
	Swap the allocation betweet $y_1 \& y_2$, the Equation \eqref{uy1} and \eqref{uy2} become
	
	\begin{equation}\label{uy1s}
	\begin{split}
		\sum_{z \in  \Com \backslash \{y_1,y_2\}}B(z|y_1) e^{-\frac{\alpha}{\mu_z} -\frac{\alpha}{\mu_{y_2}}} + B(y_2|y_1)e^{-\frac{\alpha}{\mu_{y_2}} -\frac{\alpha}{\mu_{y_1}}} \\
	+ \sum_{z \in  \Com \backslash \{y_1,y_2\}}B(y_1|z) e^{-\frac{\alpha}{\mu_z} -\frac{\alpha}{\mu_{y_2}}} + B(y_1|y_2)e^{-\frac{\alpha}{\mu_{y_2}} -\frac{\alpha}{\mu_{y_1}}} \\
	\end{split}
	\end{equation}
	
	\begin{equation}\label{uy2s}
	\begin{split}
	\sum_{z \in  \Com \backslash \{y_1,y_2\}}B(z|y_2) e^{-\frac{\alpha}{\mu_z} -\frac{\alpha}{\mu_{y_1}}} + B(y_1|y_2)e^{-\frac{\alpha}{\mu_{y_2}} -\frac{\alpha}{\mu_{y_1}}} \\
	+ \sum_{z \in  \Com \backslash \{y_1,y_2\}}B(y_2|z) e^{-\frac{\alpha}{\mu_z} -\frac{\alpha}{\mu_{y_1}}} + B(y_2|y_1)e^{-\frac{\alpha}{\mu_{y_2}} -\frac{\alpha}{\mu_{y_1}}} \\
	\end{split}
	\end{equation}

	Let's consider the difference before swap and after swap. 
	$$(\ref{uy1s})+(\ref{uy2s}) - [(\ref{uy1})+(\ref{uy2})]$$
	which is equivalent to consider the following difference
	
	\begin{equation}
	\begin{split}
	\sum_{z \in  \Com \backslash \{y_1,y_2\}}[B(y_1|z)+B(z|y_1)] e^{-\frac{\alpha}{\mu_z}} \\
	- \sum_{z \in  \Com \backslash \{y_1,y_2\}}[B(y_2|z)+B(z|y_2)] e^{-\frac{\alpha}{\mu_z}}
	\end{split}
	\end{equation}

	\begin{equation}
	\begin{split}
	\Delta_1 &= \sum_{z \in  \Com \backslash \{y_1,y_2\}}[B(y_1|z)-B(y_2|z)] e^{-\frac{\alpha}{\mu_z}}
	\end{split}
	\end{equation}
	
	\begin{equation}
	\begin{split}
	\Delta_2 &= \sum_{z \in  \Com \backslash \{y_1,y_2\}}[B(z|y_1)-B(z|y_2)] e^{-\frac{\alpha}{\mu_z}}
	\end{split}
	\end{equation}
	
	The goal is to show 
	$$\Delta_2 + \Delta_1 > 0$$
	
	\begin{lemma}\label{d1}
		$\Delta_1 > 0 $
	\end{lemma}

	\begin{lemma}\label{d1}
		$\Delta_2 > 0 $
	\end{lemma}

\end{proof}

\begin{lemma}
	$\Delta_1 > 0 $
\end{lemma}
\begin{proof}
	
	Recall $\delta$ is the distance of any consecutive agents in the content space of the community and it determine the community size and density(in term of agent number). As $\delta$ decrease, the community size and density increase. In addition, under the case without delay, by Proposition \ref{prop:production_strategy}, we have that 
	$ \sum_{z \in \Com \backslash \{y_i\}} B(y_i|z)> \sum_{z \in \Com \backslash \{y_j\}} B(y_j|z)$. Therefore, this lemma aim to establish that under the condition described, this relation is also true for the case with delay. To show this, we will use the property in $\muc^*$, $\mu(y_c|y_i) > \mu(y_c|y_j)$ if $\|y_i - \Icen\| < \|y_j - \Icen\|$. Using these results, we partition the community content interval and compare the utility of agents in each section. We will see that so long as the community is dense enough ($\delta$ small enough), then we obtain the result in the lemma.

	Let $\muc^*$ be the rate allocation vector of agents defined earlier. Without loss of generality, let's assume that content interval of the community is given by the following
	$$I_C = (-L_C, L_C) \mbox{ and } mid(I_C) = 0$$
	Then$\|y_i-\Icen \| < \|y_j-\Icen \|$ leads to three possible cases:\\
	case 1: $y_i$ and $y_j$ are in the same side of the community, (0,$L_C$)\\
	case 2: $y_i$ and $y_j$ are in the same side of the community, ($-L_C$,0)\\
	case 3: $y_i$ and $y_j$ are on different side of the community

	The proof for these three cases are similar. Therefore, we will only construct proof for one of the case above. Let's consider the case $y_i$, and $y_j$ are on the same half interval, (0,$L_C$). We can partition the community interval into the following sections:\\
	\begin{equation*}
	\begin{split}
	S_1 &= (x^*(y_j),L_C)\\
	S_2 &= (\frac{x^*(y_j)-x^*(y_i)}{2},x^*(y_j))\\
	S_3 &= (x^*(y_i),\frac{x^*(y_j)-x^*(y_i)}{2})\\
	S_4 &= (x^*(y_i)+x^*(y_j)-L_C,x^*(y_i))\\
	S_5 &= (-L_C,x^*(y_i)+x^*(y_j)-L_C)
	\end{split}
	\end{equation*}
	Then, let's consider the difference of utility in each sections above.\\
	Let $N(S_i)$ denote the set of periphery agents in the interval $S_i$, $\|N(S_i)\|$ is the number of periphery agents in $S_i$, and let $\Delta_{S_i}$ denote the difference of utility between $y_i$ and $y_j$ in interval $S_i$. Further, the $\Delta_{S_i}$ is given by 
	\begin{equation*}
	\begin{split}
	\Delta_{S_i} &=\sum_{z \in N(S_i)} [B(y_i|z)-B(y_j|z)|z)] e^{-\frac{\alpha}{\mu(y_c|z)}} \\
	&= \sum_{z \in N(S_i)} [g(x^*(y_i)|y_i)f(x^*(y_i)|z)-\\
	&\hspace{0.5inch} g(x^*(y_j)|y_i)f(x^*(y_j)|z)] e^{-\frac{\alpha}{\mu(y_c|z)}} 
	\end{split}
	\end{equation*}
	
	We will show that the overall difference of $\Delta_{S_4}$ and $\Delta_{S_1}$ is positive,i.e,
	$$\Delta_{S_4} + \Delta_{S_1} > 0$$
	
	We know that the distance between consecutive agent is the same on the interval, and by construction, we have
	$$\|S_1\| = \|S_4\|$$
	which implies 
	$$\|N(S_1)\| = \|N(S_4)\|$$
	Let $J = \|N(S_1)\| = \|N(S_4)\|$. By construction of the information community in section \ref{sec:background} and the production strategy of agent \ref{assump:production_strategy}, we know that the distance between $x^*(y_j)$ to agents in $S_1$ are multiple of $\delta$ in addition to some distance $\epsilon_{s_1}$ to the first agent, where $\epsilon_{s_1} < \delta$.
	Similarly for $S_4$. We can rewrite $\Delta_{S_1}$ and $\Delta_{S_4}$ as 
	\begin{equation*}
	\begin{split}
	\Delta_{S_1} &= - \sum_{k=0}^J [g(x^*(y_j)|y_j)f(k\delta + \epsilon_{s_1} )\\
	&-g(x^*(y_i)|y_i)f(x^*(y_j)-x^*(y_i)+k\delta + \epsilon_{s_1}) ]e^{-\frac{\alpha}{\mu(y_c|x^*(y_j)+k\delta + \epsilon_{s_1})}}
	\end{split}
	\end{equation*}
	\begin{equation*}
	\begin{split}
	\Delta_{S_4} &= \sum_{k=0}^J [g(x^*(y_i)|y_i)f(k\delta + \epsilon_{s_4})\\
	&-g(x^*(y_j)|y_j)f(x^*(y_j)-x^*(y_i)+k\delta + \epsilon_{s_4})] e^{-\frac{\alpha}{\mu(y_c|x^*(y_i)-k\delta + \epsilon_{s_4})}}
	\end{split}
	\end{equation*}
	
	Then, with the result from assumption \ref{assump:production_strategy}, we have 
	$$g(x^*(y_i)|y_i) > g(x^*(y_j)|y_j)$$
	and by lemma \ref{lemma:periphery_agent_allocation}, we have that
	$$e^{-\frac{\alpha}{\mu(y_c|x^*(y_j)+k\delta \pm \epsilon_{s_1})}}<e^{-\frac{\alpha}{\mu(y_c|x^*(y_i)-k\delta\pm \epsilon_{s_4})}}$$
	
	Since $\epsilon_{s_1}, \epsilon_{s_4} < \delta$, we can make $\delta$ small enough such that the small misalignment $\epsilon_{s_1}, \epsilon_{s_4}$ does not effect the comparison of each term in the sum. Let $\delta_0$ be be the term that satisfy this condition. In other word, if $\delta < \delta_0$, then we have the following for each term of the two sum
	\begin{equation*}
	\begin{split}
	&[g(x^*(y_i)|y_i)f(k\delta \pm \epsilon_{s_4})\\
	&-g(x^*(y_j)|y_j)f(x^*(y_j)-x^*(y_i)+k\delta + \epsilon_{s_4})] e^{-\frac{\alpha}{\mu(y_c|x^*(y_i)-k\delta + \epsilon_{s_4})}} \\
	&>\\
	&[g(x^*(y_j)|y_j)f(k\delta + \epsilon_{s_1} )\\
	&-g(x^*(y_i)|y_i)f(x^*(y_j)-x^*(y_i)+k\delta + \epsilon_{s_1}) ]e^{-\frac{\alpha}{\mu(y_c|x^*(y_j)+k\delta + \epsilon_{s_1})}}
	\end{split}
	\end{equation*}

	This means that each term in $\Delta_{S_4}$ is strictly larger than its corresponding term in $\Delta_{S_1}$. Therefore, we have
	\begin{equation}\label{s14}
	\Delta_{S_1} + \Delta_{S_4} > 0    
	\end{equation}
	
	By similar argument, we can get
	\begin{equation}\label{s23}
	\Delta_{S_2} + \Delta_{S_3} > 0    
	\end{equation}
	
	Now, let's consider the last interval $S_5$
	\begin{equation*}
	\begin{split}
	\Delta_{S_5} &= \sum_{z \in N(S_5)} [B(y_i|z)-B(y_j|z)]e^{-\frac{\alpha}{\mu(y_c|z)}} 
	\end{split}
	\end{equation*}
	Since $y_i$ is closer to agents in $N(S_5)$ than $y_j$ by construction, we have 
	$$B(y_i|z) > B(y_j|z) \text{  ,   } \forall z \in N(S_5)$$
	This immediately leas to, 
	\begin{equation}\label{s5}
	\Delta_{S_5} > 0
	\end{equation}
	
	Combining the results \ref{s14}, \ref{s23}, \ref{s5} above, we get
	$$\Delta_{S_1}+\Delta_{S_2}+\Delta_{S_3}+\Delta_{S_4}+\Delta_{S_5}>0$$
	Therefore, we obtain 
	\begin{equation*}
	\sum_{z \in \Com \backslash \{y_i\}} B(y_i|z)e^{\frac{-\alpha}{\mu(y_c|z)}}> \sum_{z \in \Com \backslash \{y_j\}} B(y_j|z)e^{\frac{-\alpha}{\mu(y_c|z)}}
	\end{equation*}
	And the result of the lemma is immediately followed from first order condition.
	
\end{proof}
