# Supplementary material for: Structure of Core-Periphery Communities
Source: arXiv:2207.06964 source file (2022-07-14)
Supplement: Supplementary file 8 [file figures.tex]

\clearpage
\onecolumn
\section{}\label{sec:figures}

\begin{figure}[H]
	\begin{minipage}{0.75\textwidth}  
		\centering
		\subfloat[Community 1]{\includegraphics[width = 0.3\linewidth]{youtube/community6_connection_scatter_size639_topcover559.png}} \quad
		\subfloat[Community 2]{\includegraphics[width = 0.3\linewidth]{youtube/community2_connection_scatter_size678_topcover610.png}} \quad
		\subfloat[Community 3]{\includegraphics[width = 0.3\linewidth]{youtube/community4_follower_connection_size724_topcover625.png}}\\ 
		\caption{Following Distribution in YouTube Communities}
		\label{fig:youtube}
	\end{minipage}      
\end{figure}

\begin{figure}[H]
	\begin{minipage}{0.55\textwidth}  
		\centering
		\subfloat[Community 1][Community 1]{\includegraphics[width = 0.45\linewidth]{twitter_ai/following_rank_scatter_ylabel.png}} \quad
		\subfloat[Community 2][Community 2]{\includegraphics[width = 0.45\linewidth]{twitter_python/following_rank_scatter_ylabel.png}}
		\caption{Following Distribution in Twitter Communities}
		\label{fig:twitter_connectivity}
	\end{minipage}
\end{figure}

\begin{figure}[h]\centering
	\begin{minipage}{0.55\textwidth}  
		\centering
		\subfloat[Community 1][Community 1]{\includegraphics[width = 0.4\linewidth]{twitter_ai/retweet_consumption.png}} \quad
		\subfloat[Community 2][Community 2]{\includegraphics[width = 0.4\linewidth]{twitter_python/retweet_consumption.png}} 
		\caption{Ranking/Ordering of Periphery Agents}
		\label{fig:twitter_core_ranking}
	\end{minipage}%
\end{figure}

\begin{figure}[H]
	\centering
	\begin{minipage}{0.55\textwidth}
		\subfloat[Community 1][Community 1]{\includegraphics[width = 0.46\linewidth]{twitter_ai/mid_rank_retweet_consumption.png}} \quad
		\subfloat[Community 2][Community 2]{\includegraphics[width = 0.46\linewidth]{twitter_python/mid_rank_retweet_consumption.png}} 
		\caption{Ranking/Ordering of Periphery Agents using Retweets of Tweets by a Random Agent}
		\label{fig:twitter_random_ranking}
	\end{minipage}
\end{figure}

\begin{figure}[H]
	\centering
	\begin{minipage}{0.55\textwidth}  
		\centering
		\subfloat[Twitter Community 1][Community 1]{\includegraphics[width = 0.45\linewidth]{twitter_ai/following_consumption.png}} \quad
		\subfloat[Twitter Community 2][Community 2]{\includegraphics[width = 0.45\linewidth]{twitter_python/following_consumption.png}}
		\caption{Correlation between number of retweets from periphery agents, and the numbers of agents followed in the community.}
		\label{fig:twitter_follower_consumption}
	\end{minipage}
\end{figure}

\begin{figure}[H]
	\centering
	\begin{minipage}{0.75\textwidth}  
	\subfloat[User ranked 3rd] {\includegraphics[width = 0.25\linewidth]{twitter_python/rank_3_local.png}}\quad
	\subfloat[User ranked 18th]{\includegraphics[width = 0.25\linewidth]{twitter_python/rank_18_local.png}}\quad
	\subfloat[User ranked 38th]{\includegraphics[width = 0.25\linewidth]{twitter_python/rank_38_local.png}}
	\caption{Connectivity between Periphery Agents in Twitter Community 2.}
	\label{fig:twitter_local_behavior2}
	\end{minipage}
\end{figure}

\begin{figure}[H]
	\centering
	\begin{minipage}{0.75\textwidth}
	\subfloat[User Ranked 3rd]{\includegraphics[width = 0.25\linewidth]{local/youtube_rank_3.png}} \quad
	\subfloat[User Ranked 180th]{\includegraphics[width = 0.25\linewidth]{local/youtube_rank_180.png}} \quad
	\subfloat[User Ranked 500th]{\includegraphics[width = 0.25\linewidth]{local/youtube_rank_500.png}}
	\caption{Connectivity between Periphery Agents in YouTube Community 3.}
	\label{fig:youtube_local}
	\end{minipage}
\end{figure}
