# Supplementary material for: Structure of Core-Periphery Communities
Source: arXiv:2207.06964 source file (2022-07-14)
Supplement: Supplementary file 9 [file Appendixoptimal_allocation_proof.tex]

\section{PROOF OF PROPOSITION \ref{prob:opt_allocation}}
In this section, we will prove proposition \ref{prob:opt_allocation} using the intermediate results we established in Appendix A. 

\begin{proof}
Let $y$ and $y'$ be arbitrary agent in the community such that 
$||y - \Cc || \leq ||y' - \Cc ||$. Let $b_0 > b_{min}$ as described in Lemma \ref{lemma:selfish_agent_allocation} and let $\delta < \delta_0$ as described in Lemma \ref{lemma:unselfish_allocation}.

In Lemma \ref{lemma:selfish_agent_allocation}, we show that under the condition $b_0 > b_{min}$, the dominant strategy(optimal allocation) of selfish agents would satisfy the structural property in proposition \ref{prob:opt_allocation},i.e. $\mu(y_0|y) \geq \mu(y_0|y')$.

With this, in lemma \ref{lemma:unselfish_allocation}, we show that if the community is dense enough,i.e. $\delta < \delta_0$, then it is optimal for unselfish agent allocate more budget to agent closer to the center of community. In other word, we have $\mu(y|y_0) \geq \mu(y'|y_0)$

This completes the proof for proposition \ref{prob:opt_allocation}
\end{proof}
