# Supplementary material for: Structure of Core-Periphery Communities
Source: arXiv:2207.06964 source file (2022-07-14)
Supplement: Supplementary file 10 [file Appendixperiphery_budget_dist_proof.tex]

\begin{lemma}\label{lemma:leaf_budget_dist}
	Let  $\muc^* = (\mu_c^*,\muc^*_p)$ be a stable allocation as given in Proposition~\ref{prop:sufficient_budget}.
	If for two periphery agents $y,y' \in \leafSet$ we have
	$||y - \Cc || < ||y' - \Cc ||$,
	then we have that  
	$$ \leafBudget - \lambda^*(y)  >   \leafBudget - \lambda^*(y').$$
\end{lemma}

\begin{proof}
    Let's start with two periphery agents $y$ and $y'$ such that 
	$$\|y - \Icen\| = \| y' - \Icen \|$$
	In this case, we have that 
	$$\leafAllocation{y} = \leafAllocation{y'},$$
	and 
	$$\lambda(y) = \lambda(y'),$$
	and
	$$\mu(y_c|y) = \mu(y_c|y').$$
	Furthermore, by first order condition as given in Eq.~\eqref{eq:leaf_foc}, we have that 
	\begin{equation*}
	S(y|y_c)e^{\frac{-\alpha}{\mu(y_c|y)}}\frac{\alpha}{\mu^2(y_c|y)} = r_0B_0e^{\frac{-\alpha}{\lambda(y)}} \frac{\alpha}{\lambda^2(y)}
	\end{equation*}
	As we move agent $y$ toward the center of community, by Proposition~\ref{lemma:core_respond}, we have that the utility of content collected by the core agent $y_c$, $S(y_c|y)$, would increase. Let's denote the increased utility agent $y$ get from the core as $S'(y_c|y)$, then we have the following.
	\begin{equation*}
	S'(y|y_c)e^{\frac{-\alpha}{\mu(y_c|y)}}\frac{\alpha}{\mu^2(y_c|y)} > r_0B_0e^{\frac{-\alpha}{\lambda(y)}} \frac{\alpha}{\lambda^2(y)}
	\end{equation*}
	For the allocation of periphery agent $y$ to be optimal, it has to satisfy the first order condition and thus, would switch to an new allocations $\mu'_p(y)$ such that  
	$$\mu'(y_c|y) > \mu(y_c|y),$$
	and
	$$\lambda'(y) < \lambda(y)$$
	Therefore, we have that 
	$$\lambda'(y) < \lambda(y) = \lambda(y')$$
	Therefore, as $y$ closer to the center of community, i.e,
	$$\|y - \Icen\| < \| y' - \Icen \|$$
	then, we have 
	$$\lambda(y) < \lambda(y').$$
	Since all periphery agents have the same budget, this leads to the result of the proposition
	$$M_p - \lambda(y) > M_p -\lambda(y').$$
\end{proof}

%\section{Proof of Proposition \ref{prop:structure}}
%Here, we show that an iterative update process, that converge to the unique stable allocation, has the structural properties given in the proposition would preserve in each iteration. Therefore, the stable allocation in the end has the same structural property. 
%\input{content/appendix/centralized_proof3.tex}
