# Supplementary material for: Structure of Core-Periphery Communities
Source: arXiv:2207.06964 source file (2022-07-14)
Supplement: Supplementary file 11 [file centralized_proof2.tex]

\newpage
\section{Global Optimization Characterize the Global Allocation}
Let $\muc$ denote the allocation of all agents in the community

\begin{equation}
    \begin{split}
          \max_{\muc}  \sum_{y \in \Com} \sum_{z \in \Com \backslash\{y\}}  [  B(z|y) e^{ - \frac{\alpha}{\mu(z|y_c)} - \frac{\alpha}{\mu(y_c|z)} }  -  c ] I(\mu(z|y_c)) + \beta \lambda(y),
    \end{split}
\end{equation}
such that
$$ \sum_{y \in \Com} \mu(y|y_c) = b_c,$$
$$ \mu(y_c|y) + \lambda(y) = B, \forall y \in \Com$$
and
$$\mu(y|y_c), \mu(z|y), \lambda(y) \geq 0.$$

\subsection{Stable Allocation}
Let $\muc^*$ be a set of allocation for all periphery agents and core agents with the following properties:

\begin{enumerate}
	\item the allocation is symmetric around core of community,i.e, if $\|y-\Icen\| =\|y' - \Icen \|$, then $\mu(y_c|y') = \mu(y_c|y)$
	\item the closer an periphery agent is to the core of community, the more rate he would allocate to the core. In other word, $\|y-\Icen\| <\|y' - \Icen \|$, then $\mu(y_c|y') > \mu(y_c|y)$
\end{enumerate}

\begin{prop}
	$\muc^*$ is the unique stable allocation if the community size is large($\delta$ is small)
\end{prop}

\begin{enumerate}
	\item The interaction between core and periphery is a potential game
	\item The utility function of potential game is strictly concave
	\item Under $\muc^*$, core agent has no incentive to change allocation if periphery agent does not change and community size is large($\delta$ is small)
	\item Under $\muc^*$, no periphery agent has incentive to change allocation if core agent does not change and community size is large($\delta$ is small)
\end{enumerate}
