# Supplementary material for: Structure of Core-Periphery Communities
Source: arXiv:2207.06964 source file (2022-07-14)
Supplement: Supplementary file 12 [file simulation.tex]

\newpage 

$$\mu(y_c) = (\mu(y_1|y_c),\mu(y_2|y_c),\mu(y_3|y_c),\mu(y_4|y_c))$$
$$\mu(y) = (\mu(y_c|y),\lambda(y))$$
\begin{equation}
\begin{split}
\max_{\mu(y_c),\{\mu(y)\}}   0.8e^{-\frac{1}{\mu(y_1|y_c)}-\frac{1}{\mu(y_c|y_1)}}+  0.6e^{-\frac{1}{\mu(y_2|y_c)}-\frac{1}{\mu(y_c|y_2)}} \\
+0.4e^{-\frac{1}{\mu(y_3|y_c)}-\frac{1}{\mu(y_c|y_3)}} +0.2e^{-\frac{1}{\mu(y_4|y_c)}-\frac{1}{\mu(y_c|y_4)}}\\
+ 0.1\lambda(y_1) + 0.1\lambda(y_2) + 0.1\lambda(y_3) + 0.1\lambda(y_4)
\end{split}
\end{equation}
such that
$$ \sum_{y \in \Com} \mu(y|y_c) = 80,$$
$$ \mu(y_c|y) + \lambda(y) = 20, \forall y \in \Com$$
and
$$\mu(y|y_c), \mu(z|y), \lambda(y) \geq 0.$$

Mapping of variable to the numerical solution
\begin{equation}
	(\mu(y_1|y_c),\mu(y_2|y_c),\mu(y_3|y_c),\mu(y_4|y_c))\\
	=(x1,x3,x5,x7)
\end{equation}

\begin{equation}
(\mu(y_c|y_1),\mu(y_c|y_2),\mu(y_c|y_3),\mu(y_c|y_4))\\
=(x2,x4,x6,x8)
\end{equation}

\begin{equation}
(\lambda(y_1),\lambda(y_2),\lambda(y_3),\lambda(y_4))\\
=(x9,x10,x11,x12)
\end{equation}
